# Supplementary material for: Medium Access Control for Dynamic Spectrum Sharing in Cognitive Radio Networks
Source: arXiv:1601.05069 source file (2016-01-19)
Supplement: Supplementary file 1 [file appendices.tex]

% Thesis statement of originality -------------------------------------

% Depending on the regulations of your faculty you may need a declaration like the one below. This specific one is from the medical faculty of the university of Dresden.

% ----------------------------------------------------------------------
